# Supplementary material for: Maintaining diversity in structured populations
Source: arXiv:2503.09841 source file (2025-09-16)
Supplement: Supplementary file 3 [file erdos-renyi.tex]

\begin{figure}[h]
    \centering
    \includegraphics[width=.95\textwidth]{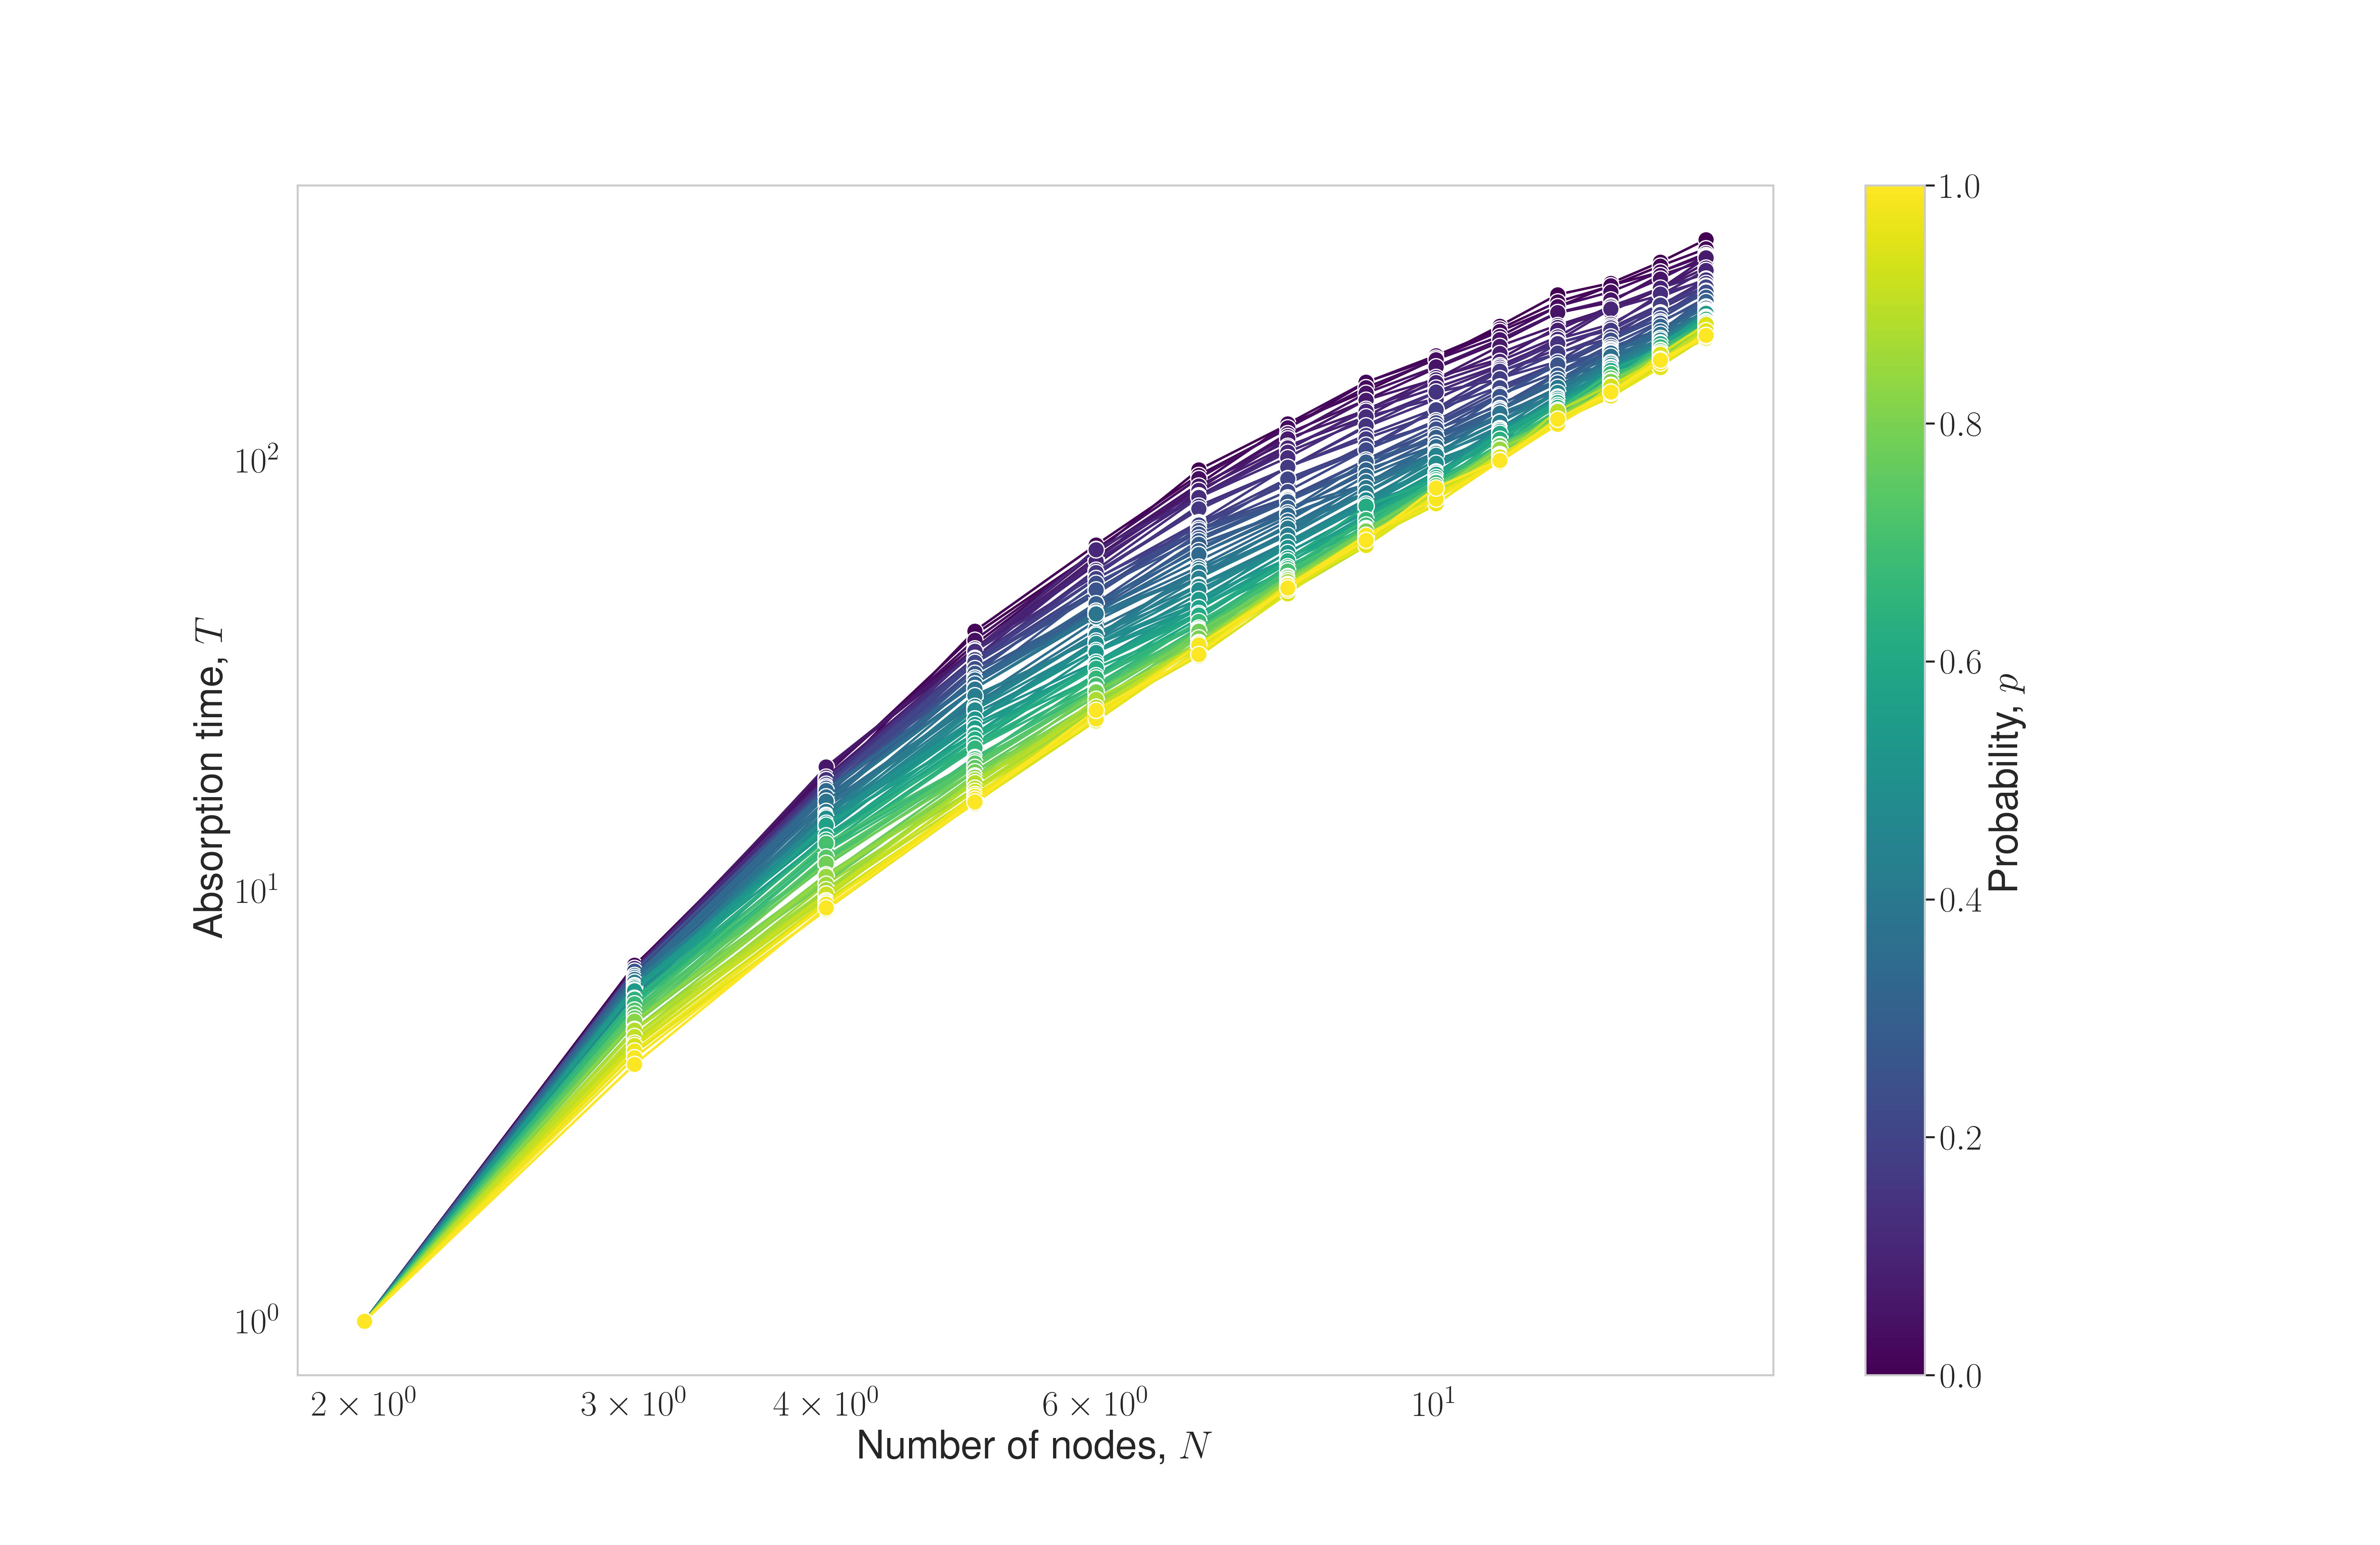}
    \caption{Absorption time ($T$) of Erd\H{o}s-Renyi random graphs $G(N, p)$ for $N=1,\ldots,15$, with $1000$ simulations per data point. For fixed $N$, we have $p$ range from $(2\log N)/N$ to $1$ in order to ensure with high probability the realized graph is connected.}
\end{figure}
