# Supplementary material for: Maintaining diversity in structured populations
Source: arXiv:2503.09841 source file (2025-09-16)
Supplement: Supplementary file 4 [file slowest.tex]

\begin{figure}[h]
    \centering
    \includegraphics[width=0.5\textwidth]{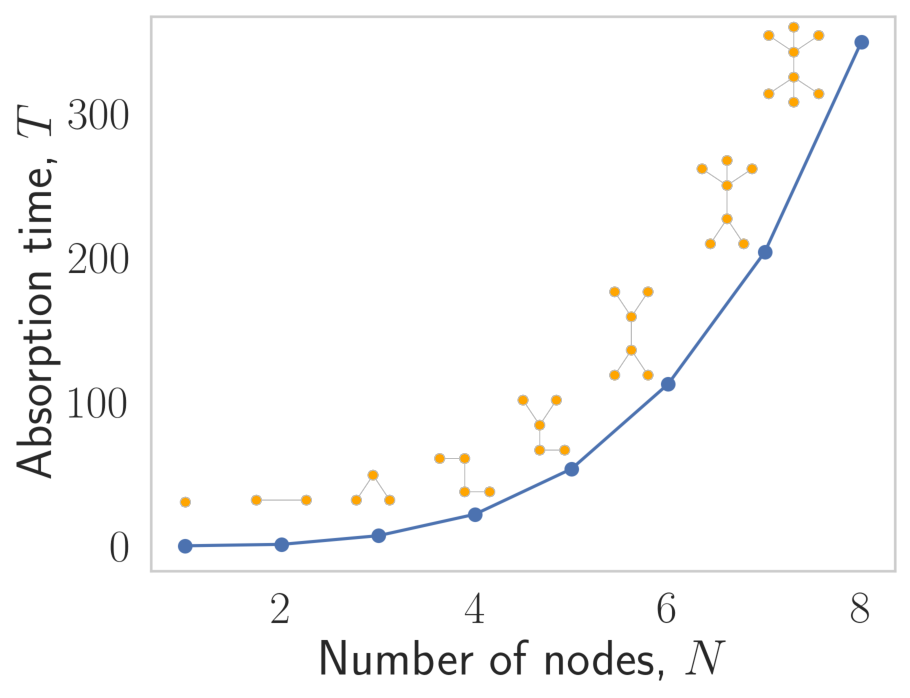}
    \caption{Absorption time ($T$) of the slowest absorbers}
\end{figure}
