# Supplementary material for: Maintaining diversity in structured populations
Source: arXiv:2503.09841 source file (2025-09-16)
Supplement: Supplementary file 5 [file trends.tex]

\begin{figure}[h]
    \centering
    \includegraphics[width=.95\textwidth]{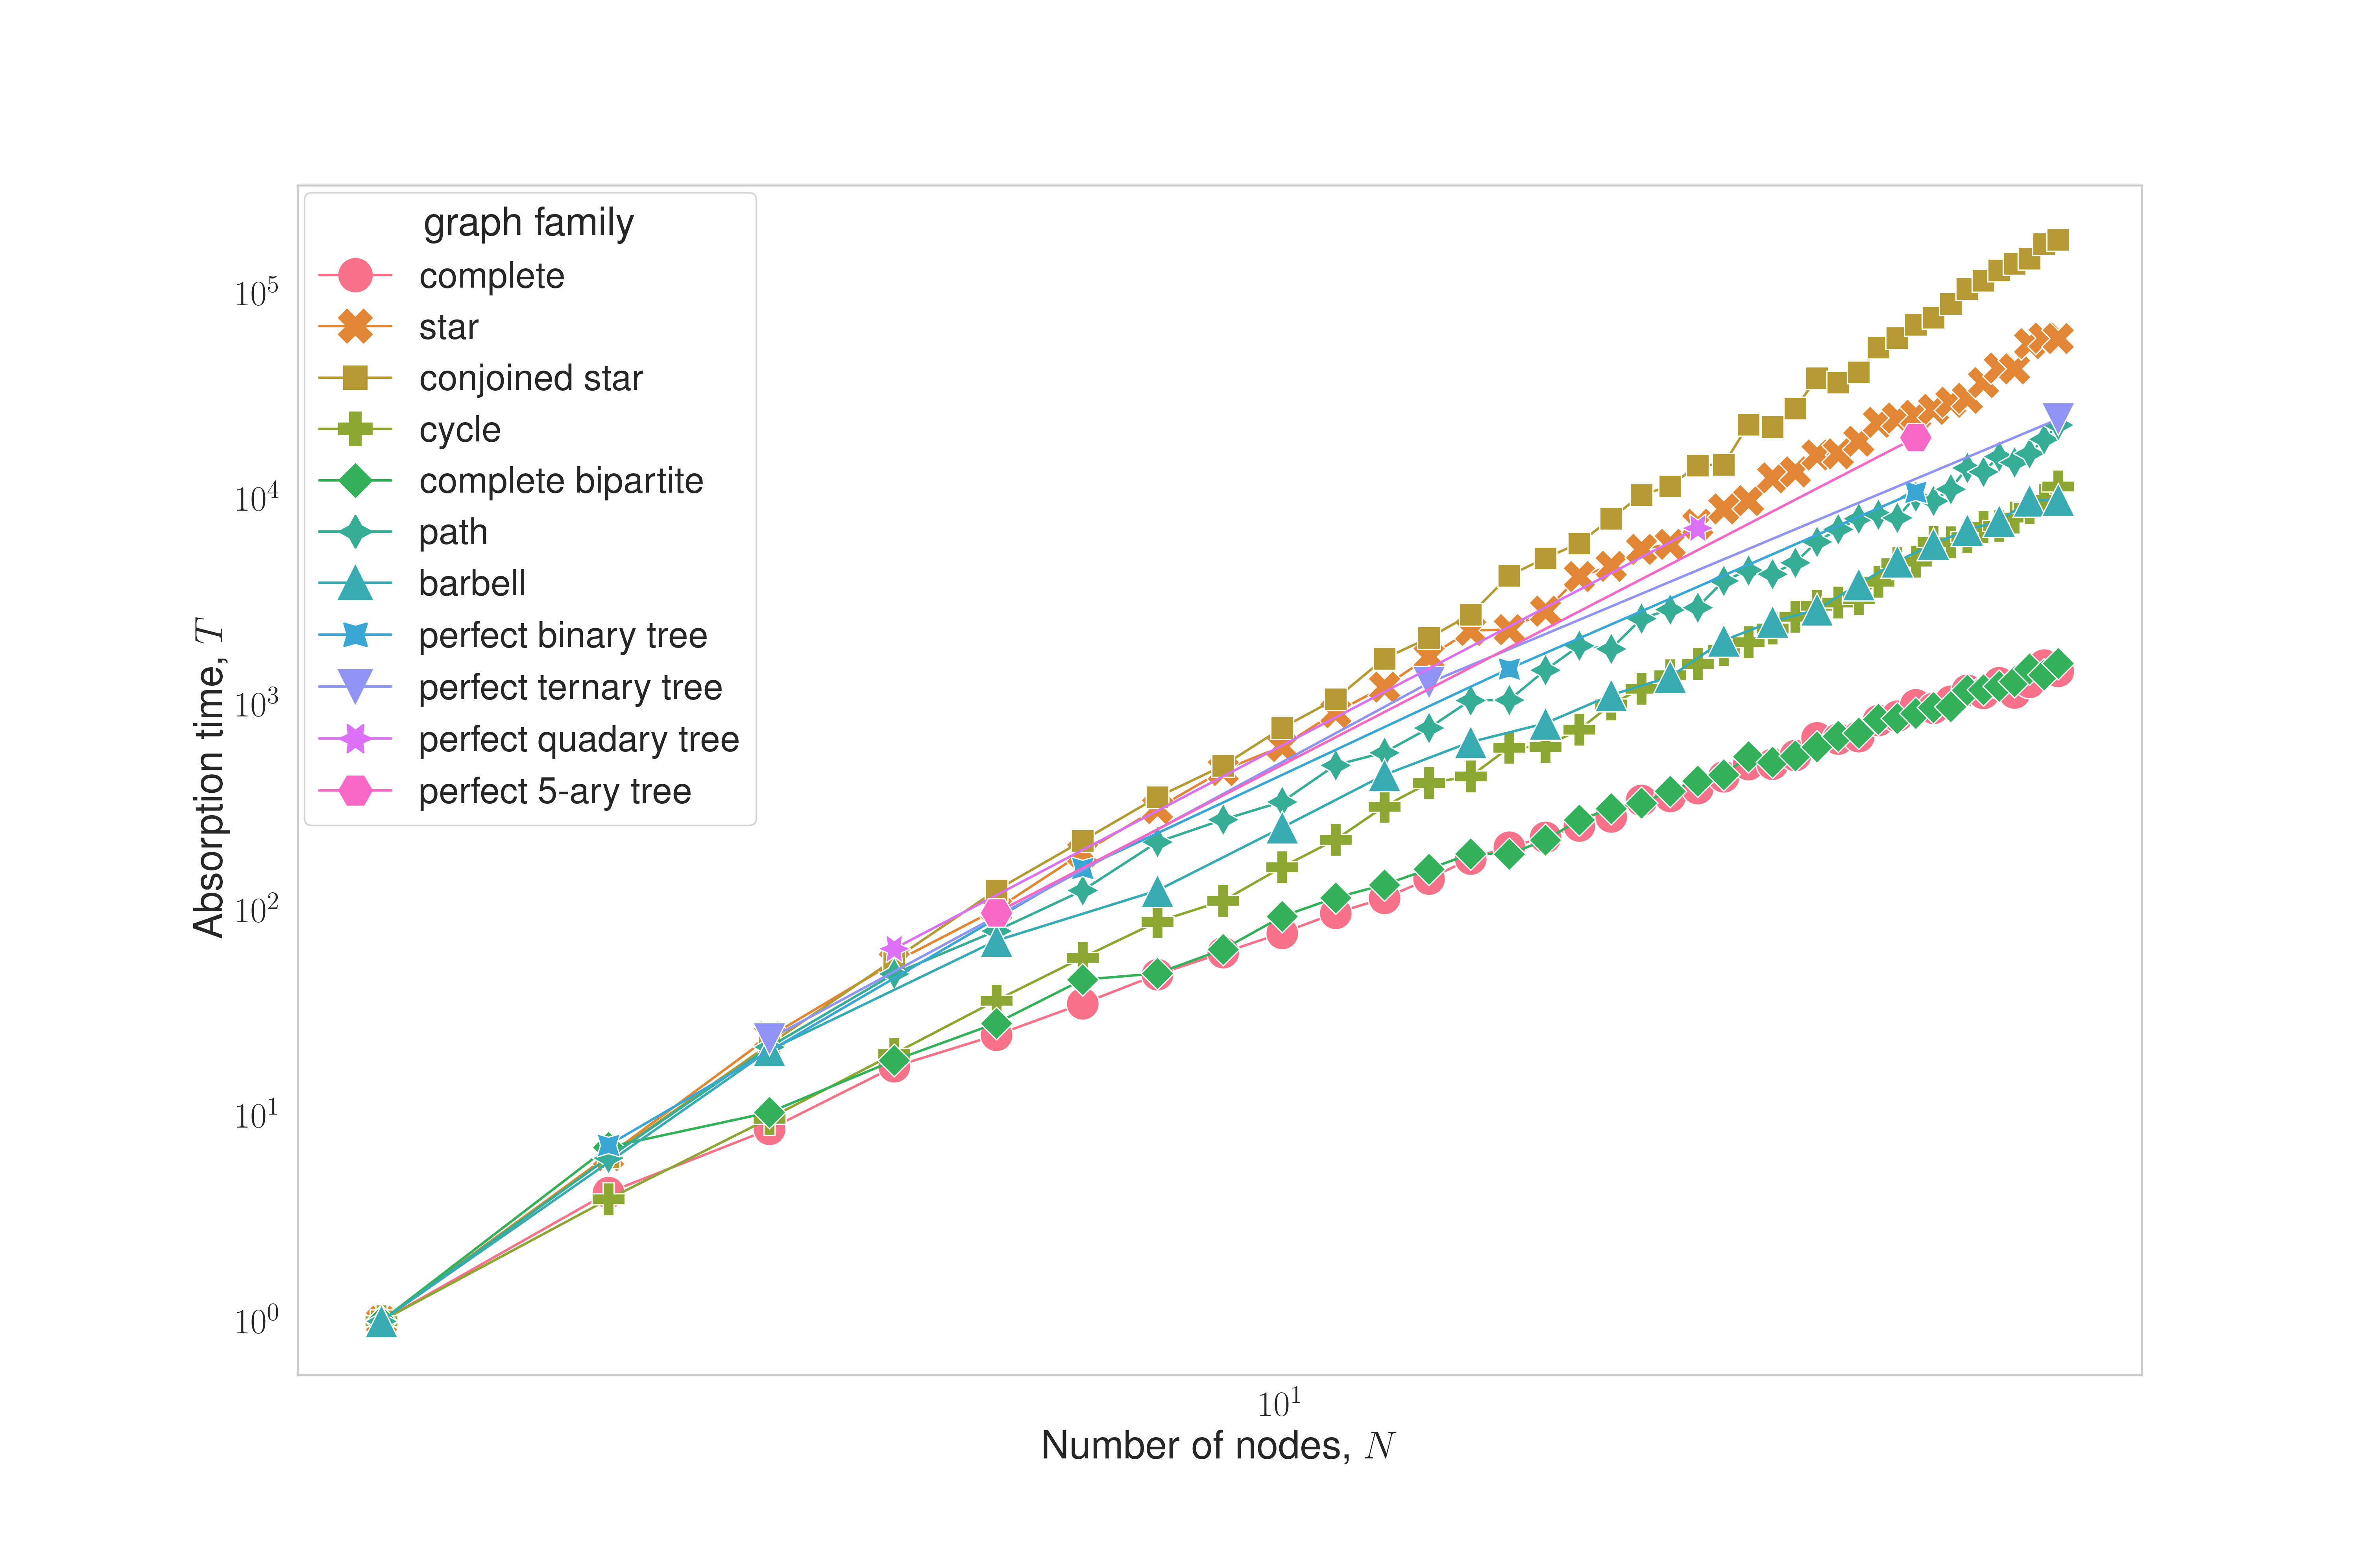}
    \caption{Absorption time ($T$) of various graph families for $N=2,\ldots,40$, with $100$ simulations per data point}
\end{figure}
