# Supplementary material for: Maintaining diversity in structured populations
Source: arXiv:2503.09841 source file (2025-09-16)
Supplement: Supplementary file 6 [file old-stuff.tex]

% \subsection{Equity potential function drift}
% Given a graph $\Graph=(\Vertices,\Edges)$
% with $|\Vertices|=N$
% a state $\omega\in\Omega$ of the multi-type
% Moran process, we define the \textit{equity} function
% $\phi\colon\Omega\to\Real_{\geq0}$
% as
% \begin{equation}
%     \phi(\omega) := N^2-\sum_{i\in[N]}(c^{\omega}_i)^2
% \end{equation}
% where $c^{\omega}_i := \#\{u\in\Vertices : \omega(u)=i\}$.
% Notice that $\phi(\omega)=0$ if and only if
% $|\omega(\Vertices)|=1$.
% For each $i\in[n]$ and $\omega\in\Omega$, let $\partial^\omega_i\colon\Vertices\to 2^{\Vertices}$
% be defined as
% \begin{equation}
%     \partial^\omega_i(u) := \{v\in\Gamma(u) : \omega(v) = i\}.
% \end{equation}
% for each $u\in\Vertices$.
% % Further, let $\partial^\omega\colon\Vertices\to 2^{\Vertices}$ be defined as
% % \begin{equation}
% %      \partial^\omega(u) := \bigcup_{\substack{i\in [n] \\ i\neq \omega(u)}}\partial^\omega_i(u).
% % \end{equation}
% We prove the following result about the
% equity potential function drift.
% \begin{theorem}\label{thm:equity-drift}
%     Let $X_0,X_1,X_2$ be a multi-type Moran process on a graph $\Graph=(\Vertices,\Edges)$ with $|\Vertices|=N$.
%     Then for each $t=0,1,2,\ldots$,
%     \begin{equation}
%         \E{\phi(X_t)-\phi(X_{t+1})\mid X_t=\omega}
%         =
%         \frac2N
%         \sum_{i\in[N]}
%         \sum_{\substack{j\in [N] \\ j\neq i}}
%         (c^{\omega}_i - c^{\omega}_j + 1)
%         \sum_{\substack{u\in\Vertices \\ \omega(u)=i}}
%         \frac{\left|\partial^{\omega}_{j}(u)\right|}{\deg(u)}.
%     \end{equation}
% \end{theorem}
% \begin{proof}
%     We have
%     \begin{align}
%          \E{\phi(X_t)-\phi(X_{t+1})\mid X_t=\omega}
%          &= \sum_{u\in\Vertices}
%          \sum_{\substack{v\in\Gamma(u)}}
%          \frac1N\cdot\frac{1}{\deg(u)}\cdot
%          (\phi(\omega)-\phi(R(\omega,v,u))) \\
%          &=
%          \sum_{i\in[N]}
%          \sum_{\substack{u\in\Vertices\\ \omega(u)=i}}
%          \sum_{\substack{v\in\Gamma(u)}}
%          \frac1N\cdot\frac{1}{\deg(u)}\cdot
%          (\phi(\omega)-\phi(R(\omega,v,u))) \\
%          &=
%          \sum_{i\in[N]}
%          \sum_{\substack{u\in\Vertices\\ \omega(u)=i}}
%          \sum_{j\in[N]}
%          \sum_{\substack{v\in\Gamma(u) \\ \omega(v)=j}}
%          \frac1N\cdot\frac{1}{\deg(u)}\cdot
%          (\phi(\omega)-\phi(R(\omega,v,u))) \\
%          &=
%          \sum_{i\in[N]}
%          \sum_{j\in[N]}
%          \sum_{\substack{u\in\Vertices\\ \omega(u)=i}}
%          \sum_{\substack{v\in\Gamma(u) \\ \omega(v)=j}}
%          \frac1N\cdot\frac{1}{\deg(u)}\cdot
%          (\phi(\omega)-\phi(R(\omega,v,u))).\label{line:drift-exact}
%     \end{align}
%     Next, 
%     if $(u,v)\in\Edges$
%     with $\omega(u)=i$ and $\omega(v)=j$ for some
%     $\omega\in\Omega$, and $i\neq j$,
%     then
%     \begin{equation}
%         \phi(R(\omega,v,u))
%         = N^2-\left(\sum_{\substack{k\in[N]\\ k\neq i,j}}(c_k^\omega)^2\right)
%         - (c_i^\omega+1)^2
%         - (c_j^\omega-1)^2.
%     \end{equation}
%     Thus
%     \begin{equation}
%         \phi(\omega) - \phi(R(\omega,v,u))
%         = -(c_i^\omega)^2
%         -(c_j^\omega)^2
%         +(c_i^\omega+1)^2
%         +(c_j^\omega-1)^2
%         = 2\cdot(c_i^\omega -c_j^\omega + 1).
%     \end{equation}
%     Continuing from \cref{line:drift-exact}
%     \begin{align}
%          \sum_{i\in[N]}
%          \sum_{j\in[N]}
%          \sum_{\substack{u\in\Vertices\\ \omega(u)=i}}
%          \sum_{\substack{v\in\Gamma(u) \\ \omega(v)=j}}
%          \frac1N\cdot\frac{1}{\deg(u)}\cdot
%          (\phi(\omega)-\phi(R(\omega,v,u)))
%          &=
%          \frac2N\sum_{i\in[N]}
%          \sum_{\substack{j\in[N] \\ j\neq i}}
%          (c_i^\omega -c_j^\omega + 1)
%          \sum_{\substack{u\in\Vertices\\ \omega(u)=i}}
%          \sum_{\substack{v\in\Gamma(u) \\ \omega(v)=j}}
%          \frac{1}{\deg(u)} \\
%          &= 
%          \frac2N\sum_{i\in[N]}
%          \sum_{\substack{j\in[N] \\ j\neq i}}
%          (c_i^\omega -c_j^\omega + 1)
%          \sum_{\substack{u\in\Vertices\\ \omega(u)=i}}
%          \frac{|\partial_j^\omega(u)|}{\deg(u)}.
%     \end{align}
% \end{proof}

% \subsection{Lower bound on expected absorption time for any graph}
% 
% \begin{theorem}
%      Let $X_0,X_1,X_2$ be a multi-type Moran process on a graph $\Graph=(\Vertices,\Edges)$ with $|\Vertices|=N$.
%     Then for each $t=0,1,2,\ldots$,
%     \begin{equation}
%         \E{\phi(X_t)-\phi(X_{t+1})\mid X_t=\omega}
%         \leq 2\cdot (N-(k-1))^2 + 4N
%     \end{equation}
%     where $k=|\omega(\Vertices)|$.
% \end{theorem}
% \begin{proof}
%     By \cref{thm:equity-drift}, we have
%     \begin{align}
%         \E{\phi(X_t)-\phi(X_{t+1})\mid X_t=\omega}
%         &= \frac2N
%         \sum_{i\in[N]}
%         \sum_{\substack{j\in [N] \\ j\neq i}}
%         (c^{\omega}_i - c^{\omega}_j + 1)
%         \sum_{\substack{u\in\Vertices \\ \omega(u)=i}}
%         \frac{\left|\partial^{\omega}_{j}(u)\right|}{\deg(u)} \\
%         &\leq \frac2N
%         \sum_{i\in[N]}
%         \sum_{\substack{j\in [N] \\ j\neq i}}
%         (c^{\omega}_i + 1)
%         \sum_{\substack{u\in\Vertices \\ \omega(u)=i}}
%         \frac{\left|\partial^{\omega}_{j}(u)\right|}{\deg(u)} \\
%         &\leq \frac2N
%         \sum_{i\in[N]}
%         \sum_{\substack{j\in [N] \\ j\neq i}}
%         (c^{\omega}_i + 1)
%         \sum_{\substack{u\in\Vertices \\ \omega(u)=i}}
%         1 \\
%         &= \frac2N
%         \sum_{i\in[N]}
%         \sum_{\substack{j\in [N] \\ j\neq i}}
%         (c^{\omega}_i + 1)\cdot c^\omega_i \\
%         &\leq 2
%         \sum_{i\in[N]}
%         (c^{\omega}_i + 1)\cdot c^\omega_i \\
%         &=2N + 2\sum_{i\in[N]} (c^{\omega}_i)^2.
%     \end{align}
%     We know that $\sum_{i\in[N]}c_i^\omega = N$.
%     By calculus, if we have $x_1,\ldots,x_k\in\Real_{\geq 1}$ such that $\sum_j x_j = m$,
%     then without loss of generality, the expression $\sum_j x_j^2$
%     is maximized when $x_1=m-k+1$ and $x_j=1$ for $j>1$.
%     Thus $\sum_{i\in[N]} (c^{\omega}_i)^2 \leq (N-(k-1))^2 + (k-1)$.
%     Bounding $k-1\leq N$ gives the desired statement.
% \end{proof}
% 
% \begin{lemma}
%     Let $\Graph=(\Vertices,\Edges)$ with $|\Vertices|=N$.
%     Let $b\colon \Real\to\Real$ be a function such that
%     \begin{equation}
%         b(z) = 2\cdot (N-(\kappa_z-1))^2 + 4N
%     \end{equation}
%     where
%     \begin{equation}
%         \kappa_z = N + \frac{1-\sqrt{1+4\cdot(N^2-z-N)}}{2}.
%     \end{equation}
%     Let $\omega\in\Omega$ with $|\omega(\Vertices)|=k$.
%     Then $b(\phi(\omega)) \geq 2\cdot (N-(k-1))^2 + 4N$.
% \end{lemma}
% \begin{proof}
%     \david{Need to flesh out argument a bit.}
%     First, it is the case that $x\geq \kappa_z-1$ if and only if
%     $N^2-z \geq (N-x)^2+x$ for all real $x$.
%     Thus $N^2-\phi(\omega) \geq (N-(k-1))^2+(k-1)$ if and only if
%     $k\geq \kappa_{\phi(\omega)}$.
%     Notice that
%     \begin{equation}
%         N^2-\phi(\omega) = \sum_{i\in[N]}(c_i^\omega)^2.
%     \end{equation}
%     The right side of the equality is upper bounded by $(N-(k-1))^2+(k-1)$
%     due to elementary calculus.
%     So if the right side is greater than $(N-(k-1))^2+(k-1)$,
%     it must be that $k\geq \kappa_{\phi(\omega)}$.
%     The conclusion follows from the fact that $b$ is monotone.
% \end{proof}

% We make use of the following lemma.
% \begin{lemma}[Corollary 15 of \cite{Kötzing_Krejca_2019}]
% \label{lemma:drift-lower}
%    Let $Z_0,Z_1,Z_2,\ldots$ be real random variables,
%    and let $\tau := \inf\{t : Z_t\leq z_{\min}\}$
%    for some $z_{\min}\geq 0$.
%    Let $D$ be the smallest real interval that contains
%    at least all values $z\geq z_{\min}$ that for all $t\leq \tau$, any $Z_t$ can take.
%    Also suppose that
%    \begin{enumerate}
%        \item $Z_0\geq z_{\min}$,
%        \item there exists some $\gamma\geq 0$ such that $|Z_{t+1}-Z_t|\leq \gamma$ for all $t$, and
%        \item there is a monotonically increasing function
%        $\beta\colon D\cup[z_{\min}-\gamma,z_{\min}]\to\Real_{>0}$
%        such that
%        \begin{itemize}
%            \item there is some value $a\geq 0$
%            such that $\beta(z+\gamma)\leq a+\beta(z-\gamma)$
%            for all possible $z$ and 
%            \item $Z_t-\E{Z_{t+1}\mid Z_0,\ldots,Z_t} \leq \beta(Z_t)$ for all $t<\tau$.
%        \end{itemize}
%    \end{enumerate}
%    Let $s = 1+\frac{a\gamma}{(a+ \beta(z_{\min}-\gamma))\beta(z_{\min}-\gamma)}$.
%    Then 
%    \begin{equation}
%        \E{\tau\mid Z_0} \geq \frac1s\cdot \int_{z_{\min}}^{Z_0} \frac{1}{\beta(y)}dy.
%    \end{equation}
% \end{lemma}
% 
% We will use the above lemma to prove the following.
% \begin{theorem}
%     Let $\Graph=(\Vertices,\Edges)$ be a graph with $|\Vertices|=N$,
%     and let $\omega\in\Omega$.
%     Then $\E {\AbsorptionTime(\Graph, \omega)} \geq (N-1)^2$.
% \end{theorem}
% 
% We provide a proof sketch.
% Given a function $\omega\in\Omega$, we define
% a scoring $\phi\colon \Omega\to \Real_{\geq0}$ of $\omega$ such that $\phi$ is only minimized when $|\omega(\Vertices)|=1$; call the set of functions that satisfy this equality $\Omega^*$.
% The way that $\phi$ is defined is such that lower scores
% are given to $\omega$ that are ``closer'' to elements of $\Omega^*$.
% Also, we will show that there is a bias for $\phi$
% towards its minimum, though the bias depends on $\omega$.
% Unfortunately, $\phi$ is not invertible, so we have to
% do some extra work to extract a possible $\omega\in\Omega$ from the results of the scoring bias,
% in order to use \cref{lemma:drift-lower}.
