# Supplementary material for: Maintaining diversity in structured populations
Source: arXiv:2503.09841 source file (2025-09-16)
Supplement: Supplementary file 7 [file 00_packages.tex]

\usepackage{tikz}
\usepackage{graphicx}
\usepackage{ifthen}
\usetikzlibrary{calc}
\usetikzlibrary{automata,positioning,fit,shapes.geometric,backgrounds}
\usepackage{amssymb,amsfonts,amsmath,amsthm}
\usepackage{caption}
\usepackage{subcaption}
\usepackage{xcolor}
\usepackage{color}   %May be necessary if you want to color links
\usepackage{hyperref}
\usepackage[capitalise]{cleveref}
\usepackage{url}
\hypersetup{
    colorlinks=true, %set true if you want colored links
    linktoc=all,     %set to all if you want both sections and subsections linked
    linkcolor=blue,  %choose some color if you want links to stand out
}



\newcommand{\eps}{\varepsilon}
\newcommand{\calO}{\mathcal{O}}


\newcommand{\fixpc}{\rho_C}
\newcommand{\fixpd}{\rho_D}

\newtheorem{theorem}{Theorem}
\newtheorem{lemma}{Lemma}
\newtheorem{definition}{Definition}
\newtheorem{observation}{Observation}
\newtheorem{question}{Question}
\newtheorem{proposition}{Proposition}
\newtheorem{corollary}{Corollary}


\newcommand{\dylan}[1]{{\color{blue} \textrm{Dylan says: }#1}}
\newcommand{\martin}[1]{{\color{purple} \textrm{Martin says: }#1}}
\newcommand{\david}[1]{{\color{olive} \textrm{David says: }#1}}
\newcommand{\jakub}[1]{{\color{orange} \textrm{Jakub says: }#1}}
\newcommand{\pepa}[1]{{\color{teal} \textrm{Pepa says: }#1}}












\usepackage{amsfonts}
\usepackage{amsmath}
\usepackage{amssymb}
\usepackage{amsthm}
\usepackage{bbm}
\usepackage{graphicx} 
\usepackage{mathrsfs}
\usepackage{float}
\usepackage{caption}
\usepackage{subcaption}
\usepackage{graphicx}

\usepackage{fullpage}
% \pagestyle{empty}
\usepackage[margin=0.5in]{geometry}
\usepackage{xcolor}
\usepackage{caption}
\usepackage{authblk}
\usepackage{graphbox}

\usepackage{cite}
\usepackage{lipsum} 
\usepackage[title]{appendix}
\usepackage[right]{lineno}
\usepackage{enumitem}


%%%%%% Commands
% \newcommand{\Graph}{\ensuremath{\mathsf{G}}}
% \newcommand{\Vertices}{\ensuremath{\mathsf{V}}}
% \newcommand{\Edges}{\ensuremath{\mathsf{E}}}
\newcommand{\Graph}{\ensuremath{G}}
\newcommand{\Vertices}{\ensuremath{V}}
\newcommand{\Edges}{\ensuremath{E}}

\newcommand{\Real}{\ensuremath{\mathbb{R}}}
\newcommand{\Natural}{\ensuremath{\mathbb{N}}}

% TODO: replace this with the actual condition.
\newcommand{\Condition}{\ensuremath{\mathscr{C}}}

\newcommand{\Degree}{\ensuremath{\mathrm{deg}}}
\newcommand{\InDegree}[1]{\ensuremath{\Degree^-(#1)}}
\newcommand{\OutDegree}[1]{\ensuremath{\Degree^+(#1)}}
\newcommand{\VertexDegree}[1]{\ensuremath{\Degree(#1)}}
\newcommand{\VertexAverageDegreeOfIncoming}[1]{\ensuremath{\widetilde{\Degree}(#1)}}

\newcommand{\STG}[1]{\ensuremath{\mathsf{STG}(#1)}}

\newcommand{\FixationProbability}{\ensuremath{\mathrm{fp}}}
\newcommand{\FixationProbabilityUnderNeutralEvolution}[1]{\ensuremath{\FixationProbability(#1)}}
\newcommand{\AbsorptionTime}{\ensuremath{\mathrm{AT}}}

\newcommand{\SymmetricDifference}{\triangle\,}
\newcommand{\R}{\ensuremath{\mathbb{R}}}
\newcommand{\N}{\ensuremath{\mathbb{N}}}
\newcommand{\Mutants}{\ensuremath{\mathscr{S}}}
\newcommand{\Fixates}{\ensuremath{\mathcal{F}}}

\newcommand{\e}{\varepsilon}
\newcommand{\Set}[1]{\{#1\}}
\newcommand{\E}[1]{\ensuremath{\mathbb{E}\left[#1\right]}}
\newcommand{\Var}[1]{\ensuremath{\mathrm{Var}\left[#1\right]}}

\newcommand{\poly}{\text{poly}}

\newcommand{\bx}{\ensuremath{\mathbf{x}}}

\newcommand{\Types}{\ensuremath{\mathbb{T}}}
\newcommand{\Event}{\ensuremath{\mathcal{E}}}


\let\savedleq=\leq % save them in case you ever want them
\let\savedgeq=\geq %
\let\savedle=\le % save them in case you ever want them
\let\savedge=\ge %
\let\leq=\leqslant % redefine them
\let\geq=\geqslant %
\let\le=\leqslant % redefine them
\let\ge=\geqslant %

\def\deg{\operatorname{deg}}

\def\indeg{\deg^-}
\def\outdeg{\deg^+}


\crefname{claim}{claim}{claims}

\def\T{\operatorname{T}}
\def\AT{\operatorname{AT}}
\def\FT{\T}
\def\ET{\operatorname{ExtT}}
\def\ATr{\AT_r}
\def\FTr{\FT_r}
\def\ETr{\ET_r}
% \def\twolayer{\operatorname{TL}}
\def\fp{\mathrm{fp}}
\def\fpr{\mathrm{fp}_r}
%\def\twolayer{\operatorname{TL}}
\def\twolayer{G}
\newcommand\pmin{\fp_{\rm min}}
\newcommand\pmax{\fp_{\rm max}}
\newcommand\fpmin{\pmin}
\newcommand\fpminr{\pmin_{(r)}}
\newcommand\fpmax{\pmax}
\def\good{balanced}
\def\short{fast}

\def\pup{p_r^+}
\def\pdown{p_r^-}
\def\bias{\gamma_r}
\def\eps{\varepsilon}
