# Supplementary material for: Maintaining diversity in structured populations
Source: arXiv:2503.09841 source file (2025-09-16)
Supplement: Supplementary file 8 [file complete_graph.tex]

\section{Complete graph}

For every configuration $c$ on $K_n$, we define a potential $p(c)$ that computes the number of edges that have different mutants.

\begin{lemma}
    We have $E[p(c') | p(c) \text{ and the step is active}] = p(c)-1$ and 
    $E[p(c') | p(c)] = p(c)-\frac{p(c)}{\binom{n}{2}}$
\end{lemma}
\begin{proof}
    If the step is active, we can imagine a different dynamic: First, a random edge between two different types is selected and then a random endpoint of the edge reproduces.

    For an edge between two types $1$ and $2$ with sizes $k$ and $k'$, if the first type reproduces, we are left with $k+1$ and $k'-1$ of type $1$ and $2$ respectively.
    In that case, the number of edges between different types changes as $-k + (k'-1)$.
    If the second type reproduces, the change is $-k' + (k-1)$.
    That means conditioned that the reproduction happens over the edge, we have
    $\frac{1}{2}(-k + k'-1) + \frac{1}{2} (-k' + k-1) = -1$.
    This holds for every edge between any two types, which means we have a supermartingale.

    Where the second is the consequence of the fact that $\frac{p(c)}{\binom{n}{2}}$ is the probability of making an active step.
\end{proof}


\subsection{Mutation}

We suppose that the mutation can happen with a small probability in every reproduction.
In the potential, it is expressed in the following way:
\begin{lemma}\label{lemm:mutation_potential}
    With mutation $x$, we have
    $E[p(c') | p(c)] = (1-x)p(c)(1-\frac{1}{\binom{n}{2}}) + x(p(c) + n -1 - \frac{p(c)}{n})$.
\end{lemma}
\begin{proof}
    With probability $1-x$ no mutation happens, if the mutation happens, we add all newly created diverse edges.
    The number of them is $n-1$ minus the average number of diverse edges of a vertex.
\end{proof}

Using \Cref{lemm:mutation_potential}, we can compute the number of diverse edges for given $x$.
For instance for $x = 1/n$, we have $p(c) = \frac{2}{3}\binom{n}{2}$. 
On the other hand, having $1/10$ of the edges be diverse, we need $x = \frac{1}{8n-7}$.
