# Supplementary material for: Maintaining diversity in structured populations
Source: arXiv:2503.09841 source file (2025-09-16)
Supplement: Supplementary file 9 [file general_bounds.tex]

\section{General bounds}

Let $d$ be the maximal degree and $d'$ the minimal degree.

\begin{theorem}
    For all graphs, the time to fixation is $\calO(\frac{n^3d^3}{d'^2})$.
\end{theorem}
